# Supplementary material for: Neural Novel Actor: Learning a Generalized Animatable Neural Representation for Human Actors
Source: arXiv:2208.11905 source file (2023-05-23)
Supplement: Supplementary file 1 [file 0_authors.tex]

%%%%%%%%%%%%
% INITIAL SUBMISSION 
%\begin{comment}
% The \author macro works with any number of authors. There are two commands
% used to separate the names and addresses of multiple authors: \And and \AND.
%
% Using \And between authors leaves it to LaTeX to determine where to break the
% lines. Using \AND forces a line break at that point. So, if LaTeX puts 3 of 4
% authors names on the first line, and the last on the second line, try using
% \AND instead of \And before the third author name.

\begin{comment}
    \titlerunning{Neural Novel Actor}
    % If the paper title is too long for the running head, you can set
    % an abbreviated paper title here
    %
    \author{First Author\inst{1}\orcidID{0000-1111-2222-3333} \and
    Second Author\inst{2,3}\orcidID{1111-2222-3333-4444} \and
    Third Author\inst{3}\orcidID{2222--3333-4444-5555}}
    %
    \authorrunning{F. Author et al.}
    % First names are abbreviated in the running head.
    % If there are more than two authors, 'et al.' is used.
    %
    \institute{Princeton University, Princeton NJ 08544, USA \and
    Springer Heidelberg, Tiergartenstr. 17, 69121 Heidelberg, Germany
    \email{lncs@springer.com}\\
    \url{http://www.springer.com/gp/computer-science/lncs} \and
    ABC Institute, Rupert-Karls-University Heidelberg, Heidelberg, Germany\\
    \email{\{abc,lncs\}@uni-heidelberg.de}}
\end{comment}
\author{%
  David S.~Hippocampus\thanks{Use footnote for providing further information
    about author (webpage, alternative address)---\emph{not} for acknowledging
    funding agencies.} \\
  Department of Computer Science\\
  Cranberry-Lemon University\\
  Pittsburgh, PA 15213 \\
  \texttt{hippo@cs.cranberry-lemon.edu} \\
  % examples of more authors
  % \And
  % Coauthor \\
  % Affiliation \\
  % Address \\
  % \texttt{email} \\
  % \AND
  % Coauthor \\
  % Affiliation \\
  % Address \\
  % \texttt{email} \\
  % \And
  % Coauthor \\
  % Affiliation \\
  % Address \\
  % \texttt{email} \\
  % \And
  % Coauthor \\
  % Affiliation \\
  % Address \\
  % \texttt{email} \\
}

%\end{comment}
%******************
