# Supplementary material for: Neural Novel Actor: Learning a Generalized Animatable Neural Representation for Human Actors
Source: arXiv:2208.11905 source file (2023-05-23)
Supplement: Supplementary file 3 [file x_document_args.tex]

% \renewcommand\thelinenumber{\color[rgb]{0.2,0.5,0.8}\normalfont\sffamily\scriptsize\arabic{linenumber}\color[rgb]{0,0,0}}
% \renewcommand\makeLineNumber {\hss\thelinenumber\ \hspace{6mm} \rlap{\hskip\textwidth\ \hspace{6.5mm}\thelinenumber}}
% \linenumbers
\pagestyle{headings}
\mainmatter
  % Insert your submission number here

% CAMERA READY SUBMISSION
\begin{comment}
    \titlerunning{Neural Novel Actor}
    % If the paper title is too long for the running head, you can set
    % an abbreviated paper title here
    %
    \author{First Author\inst{1}\orcidID{0000-1111-2222-3333} \and
    Second Author\inst{2,3}\orcidID{1111-2222-3333-4444} \and
    Third Author\inst{3}\orcidID{2222--3333-4444-5555}}
    %
    \authorrunning{F. Author et al.}
    % First names are abbreviated in the running head.
    % If there are more than two authors, 'et al.' is used.
    %
    \institute{Princeton University, Princeton NJ 08544, USA \and
    Springer Heidelberg, Tiergartenstr. 17, 69121 Heidelberg, Germany
    \email{lncs@springer.com}\\
    \url{http://www.springer.com/gp/computer-science/lncs} \and
    ABC Institute, Rupert-Karls-University Heidelberg, Heidelberg, Germany\\
    \email{\{abc,lncs\}@uni-heidelberg.de}}
\end{comment}
%******************
