# Supplementary material for: Neural Novel Actor: Learning a Generalized Animatable Neural Representation for Human Actors
Source: arXiv:2208.11905 source file (2023-05-23)
Supplement: Supplementary file 4 [file x_preamble.tex]

%%%%%%%%%%%%%%%%%%%%%%%%%%%%%%%%%%%%%%%%%%%%%%%%%
% common preambles
%%%%%%%%%%%%%%%%%%%%%%%%%%%%%%%%%%%%%%%%%%%%%%%%%

\usepackage{graphicx}
% DO NOT USE \usepackage{times}, it will be removed by typesetters
%\usepackage{times}

\usepackage{tikz}
\usepackage{comment}
\usepackage{amsmath,amssymb} % define this before the line numbering.
\usepackage{color}
\usepackage{ulem}

% The "axessiblity" package can be found at: https://ctan.org/pkg/axessibility?lang=en
\usepackage[accsupp]{axessibility}  % Improves PDF readability for those with disabilities.

%--------------------------------------------------
% colored text and comments
%--------------------------------------------------
\usepackage{bm}
\newcommand{\blue}[1]{\textcolor{blue}{{#1}}}
\newcommand{\LJ}[1]{{\textcolor{blue}{[\textbf{LJ:} #1]}}}
\newcommand{\libin}[1]{\textcolor{blue}{[libin]:#1}}
\newcommand{\llb}[1]{\textcolor{blue}{#1}}
\newcommand{\lbDel}[1]{\textcolor{blue}{\sout{#1}}}
\newcommand{\qingzhe}[1]{\textcolor{red}{[qingzhe]:#1}}
\newcommand{\yiming}[1]{\textcolor{red}{[yiming]:#1}}


\renewcommand{\blue}[1]{{{#1}}}
\renewcommand{\LJ}[1]{{#1}}
\renewcommand{\libin}[1]{#1}
\renewcommand{\llb}[1]{#1}
\renewcommand{\lbDel}[1]{}
\renewcommand{\qingzhe}[1]{#1}
\renewcommand{\yiming}[1]{#1}

%--------------------------------------------------
% for vectors (should be surrounded by $)
%--------------------------------------------------
%\usepackage{graphicx}
%\usepackage{subcaption}
\usepackage{multirow}
%\usepackage{mathtools}
\usepackage{mathrsfs}
\newcommand{\isep}{\mathrel{{.}\,{.}}\nobreak}
\newcommand{\vect}[1]{{\bm{#1}}}
\newcommand{\unit}[1]{\widehat{#1}}
\newcommand{\sign}[1]{\operatorname{sign}(#1)}
\newcommand{\vecangle}[2]{(#1,#2)}

%--------------------------------------------------
% common shortcuts in the text
%--------------------------------------------------
\usepackage{xspace}
\newcommand{\ie}{\textsl{i.e.}~}
\newcommand{\eg}{\textsl{e.g.}~}
\newcommand{\etal}{\textsl{et~al.}~}
\newcommand{\wrt}{\textsl{w.r.t.}~}
\newcommand{\NB}{\textsl{NB:}~}
\newcommand{\vs}{\textsl{vs.}~}
\newcommand{\cf}{\textsl{cf.}~}
\newcommand{\resp}{respectively\xspace}
\newcommand{\aka}{\textsl{a.k.a.}~}


%--------------------------------------------------
% Commands for keeping text (it's in the latex
%  but not displayed on pdf)
%--------------------------------------------------
\newcommand{\keep}[1]{}
\newcommand{\old}[1]{}

%--------------------------------------------------
% Math operators
%--------------------------------------------------
\DeclareMathOperator*{\argmin}{arg\,min}
\DeclareMathOperator*{\softmax}{softmax}
\DeclareMathOperator*{\GCN}{GCN}
\DeclareMathOperator*{\CNN}{CNN}
\DeclareMathOperator*{\MLP}{MLP}
\DeclareMathOperator*{\DeGCN}{GCN*}
\DeclareMathOperator*{\FwdSkin}{\mathcal{F}}
\DeclareMathOperator*{\BwdSkin}{\mathcal{G}}


% Recommended, but optional, packages for figures and better typesetting:
\usepackage{times}
\usepackage{epsfig}
\usepackage{microtype}
\usepackage{graphicx}
\usepackage{subfigure}
\usepackage{booktabs} % for professional tables
% \usepackage{subfig}

% hyperref makes hyperlinks in the resulting PDF.
% If your build breaks (sometimes temporarily if a hyperlink spans a page)
% please comment out the following usepackage line and replace
% \usepackage{icml2021} with \usepackage[nohyperref]{icml2021} above.
\usepackage{hyperref}
% Attempt to make hyperref and algorithmic work together better:
\newcommand{\theHalgorithm}{\arabic{algorithm}} 
\newcommand{\eqnref}[1]{{Equation~{#1}}}
\newcommand{\figref}[1]{{Figure~{#1}}}
