# Supplementary material for: Neural Novel Actor: Learning a Generalized Animatable Neural Representation for Human Actors
Source: arXiv:2208.11905 source file (2023-05-23)
Supplement: Supplementary file 5 [file x_template_args.tex]

% if you need to pass options to natbib, use, e.g.:
%     \PassOptionsToPackage{numbers, compress}{natbib}
% before loading neurips_2022


% ready for submission
% \usepackage{neurips_2022}
\usepackage[nonatbib]{neurips_2022}

% to compile a preprint version, e.g., for submission to arXiv, add add the
% [preprint] option:
%     \usepackage[preprint]{neurips_2022}


% to compile a camera-ready version, add the [final] option, e.g.:
%     \usepackage[final]{neurips_2022}


% to avoid loading the natbib package, add option nonatbib:
% \usepackage[nonatbib]{neurips_2022}
\usepackage[pdftex]{graphicx}

\usepackage[utf8]{inputenc} % allow utf-8 input
\usepackage[T1]{fontenc}    % use 8-bit T1 fonts
\usepackage{hyperref}       % hyperlinks
\usepackage{url}            % simple URL typesetting
\usepackage{booktabs}       % professional-quality tables
\usepackage{amsfonts}       % blackboard math symbols
\usepackage{nicefrac}       % compact symbols for 1/2, etc.
\usepackage{microtype}      % microtypography
\usepackage{xcolor}         % colors
% \usepackage{subcaption}
\usepackage{subfigure}
\usepackage{amssymb}
\usepackage{bbding}
\usepackage{pifont}
\usepackage{caption} 
\captionsetup[table]{skip=8pt}
% \usepackage{caption}
